# Supplementary material for: Theoretical and numerical comparison of quantum- and classical embedding models for optical spectra
Source: arXiv:2304.11682 ancillary file (2023-04-23)
Supplement: Supplementary file 1 [file si.pdf]

# Supporting information to:

# Theoretical and numerical comparison of quantum- and classical embedding models for optical spectra

Marina Jansen, Peter Reinholdt, Erik D. Hedegård, and Carolin König

# S-1 Preliminary remarks

In this supporting information, the calculated excitation energies (in eV) and oscillator strengths for the models `NOPOL`, `GSPOL` and `PE DPOL` introduced in section 2 in the main text of the strongest $\pi \to \pi^*$ transition are given. Calculations were done with `PE` and `FDE` embedding models according to the procedure presented in section 3 of the main text for different configurations of pNA and pFTAA. For the definition of the different shifts ($\Delta$`NOPOL`, $\Delta$`GSPOL`, $\Delta$`DPOL`, $\Delta$ `DPOL+EEF`, and $\Delta$`REF`) as well as contributions ($\Delta$`NOPOL`, $\Delta\Delta$`GSPOL`, $\Delta\Delta$`DPOL`, $\Delta\Delta$`DPOL+EEF`, and $\Delta\Delta$ `EEF`) we refer to the main text.

# S-2 Excitation energies and $\mathcal{S}$-Shifts for *para*-Nitroaniline

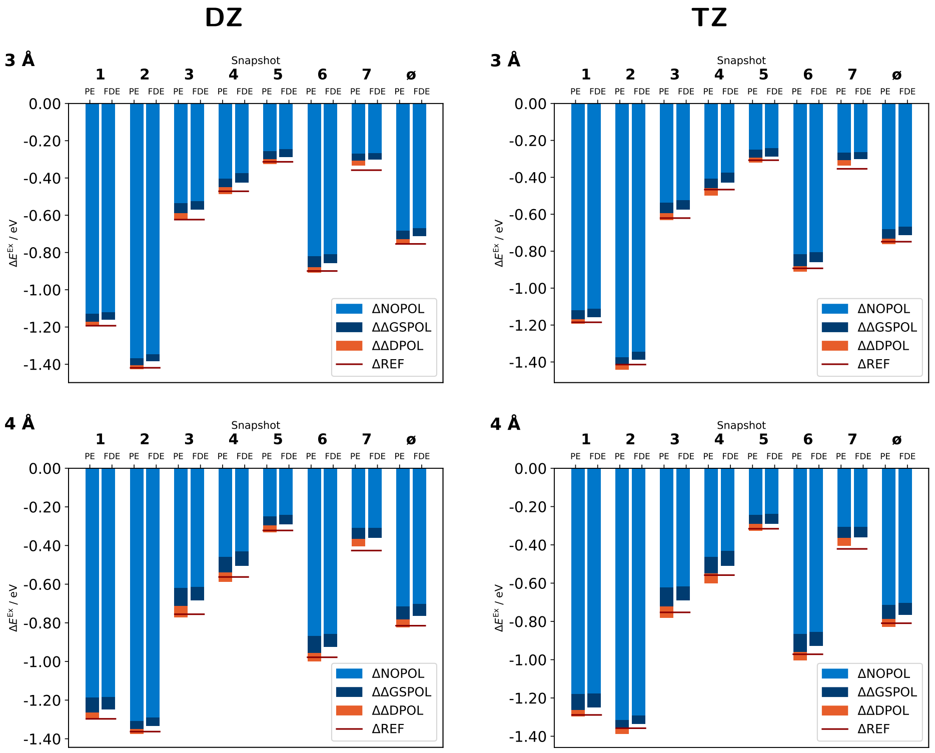


**Figure S-2.1:** Contributions to the $\mathcal{S}$-shifts and their average for different configurations of pNA in 3 and 4 Å water environments of water obtained from a MD simulation and subsequently calculated in a `PE` and `FDE` framework and different orders of polarization contributions obtained in calculations with aug-cc-pVDZ and aug-cc-pVTZ basis sets.

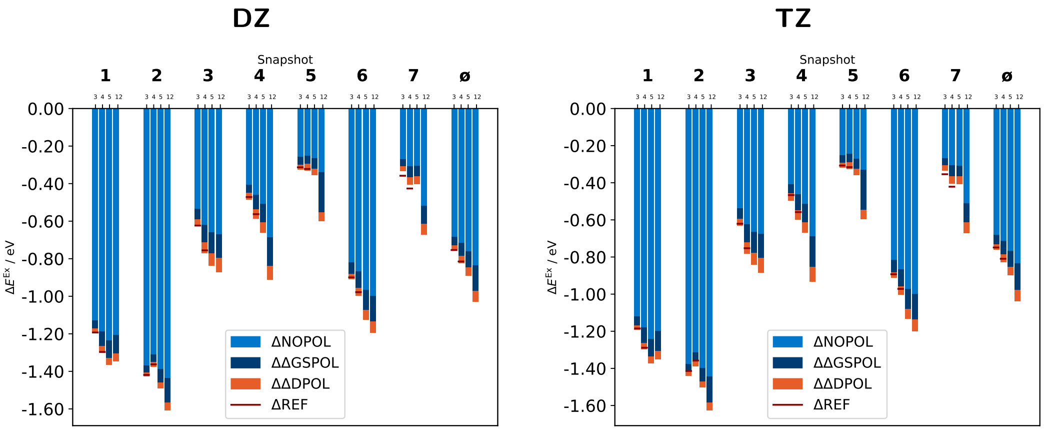


**Figure S-2.2:** Contributions to the $\mathcal{S}$-shifts and their average for different configurations of pNA in 3, 4,5 and 12 Å environments of water obtained from a MD simulation and subsequently calculated in a `PE` framework and different orders of polarization contributions obtained in calculations with aug-cc-pVDZ and aug-cc-pVTZ basis sets.

## S-2.1 Calculations in a 3 Å water environment

**Table S-2.1:** Excitation energies and contributions from the different polarization models to the $\mathcal{S}$-shifts and their average for different configurations of pNA in aug-cc-pVDZ quality and a 3 Å water environment obtained with a FDE embedding model.

| $\Delta E^{\text{ex}}$(FDE): | VACUUM | NOPOL | Δ NOPOL | GSPOL | ΔΔ GSPOL | ΔGSPOL | ΔDPOL | REF | Δ REF |
|---|---|---|---|---|---|---|---|---|---|
| Snap 1 | 4.68 | 3.56 | -1.12 | 3.52 | -0.04 | -1.16 | -1.16 | 3.48 | -1.19 |
| Snap 2 | 4.51 | 3.17 | -1.35 | 3.13 | -0.04 | -1.38 | -1.38 | 3.09 | -1.42 |
| Snap 3 | 4.19 | 3.66 | -0.52 | 3.62 | -0.05 | -0.57 | -0.57 | 3.56 | -0.62 |
| Snap 4 | 4.01 | 3.64 | -0.37 | 3.59 | -0.05 | -0.42 | -0.42 | 3.54 | -0.47 |
| Snap 5 | 4.25 | 4.01 | -0.24 | 3.97 | -0.04 | -0.29 | -0.29 | 3.94 | -0.31 |
| Snap 6 | 4.54 | 3.73 | -0.81 | 3.68 | -0.05 | -0.86 | -0.86 | 3.64 | -0.90 |
| Snap 7 | 4.53 | 4.26 | -0.27 | 4.23 | -0.03 | -0.30 | -0.30 | 4.17 | -0.36 |
| ∅ | 4.39 | 3.72 | -0.67 | 3.67 | -0.04 | -0.71 | -0.71 | 3.63 | -0.75 |

**Table S-2.2:** Excitation energies and contributions from the different polarization models to the $\mathcal{S}$-shifts and their average for different configurations of pNA in aug-cc-pVDZ quality and a 3 Å water environment obtained with a PE embedding model.

| $\Delta E^{\text{ex}}$(PE): | VACUUM | NOPOL | Δ NOPOL | GSPOL | ΔΔ GSPOL | DPOL | ΔΔ DPOL | ΔGSPOL | ΔDPOL | REF | Δ REF |
|---|---|---|---|---|---|---|---|---|---|---|---|
| Snap 1 | 4.68 | 3.55 | -1.13 | 3.50 | -0.04 | 3.48 | -0.02 | -1.17 | -1.19 | 3.48 | -1.19 |
| Snap 2 | 4.51 | 3.14 | -1.37 | 3.11 | -0.04 | 3.09 | -0.02 | -1.41 | -1.43 | 3.09 | -1.42 |
| Snap 3 | 4.19 | 3.65 | -0.53 | 3.60 | -0.06 | 3.56 | -0.04 | -0.59 | -0.63 | 3.56 | -0.62 |
| Snap 4 | 4.01 | 3.61 | -0.40 | 3.56 | -0.04 | 3.53 | -0.04 | -0.45 | -0.49 | 3.54 | -0.47 |
| Snap 5 | 4.25 | 3.99 | -0.26 | 3.95 | -0.04 | 3.93 | -0.03 | -0.30 | -0.32 | 3.94 | -0.31 |
| Snap 6 | 4.54 | 3.72 | -0.82 | 3.66 | -0.06 | 3.63 | -0.03 | -0.88 | -0.91 | 3.64 | -0.90 |
| Snap 7 | 4.53 | 4.26 | -0.27 | 4.22 | -0.04 | 4.19 | -0.03 | -0.31 | -0.33 | 4.17 | -0.36 |
| ∅ | 4.39 | 3.70 | -0.68 | 3.66 | -0.05 | 3.63 | -0.03 | -0.73 | -0.76 | 3.63 | -0.75 |

**Table S-2.3:** Excitation energies and contributions from the different polarization models to the $\mathcal{S}$-shifts and their average for different configurations of pNA in aug-cc-pVTZ quality and a 3 Å water environment obtained with a FDE embedding model.

| $\Delta E^{\text{ex}}$(FDE): | VACUUM | NOPOL | Δ NOPOL | GSPOL | ΔΔ GSPOL | ΔGSPOL | ΔDPOL | REF | Δ REF |
|---|---|---|---|---|---|---|---|---|---|
| Snap 1 | 4.68 | 3.57 | -1.11 | 3.53 | -0.04 | -1.16 | -1.16 | 3.50 | -1.19 |
| Snap 2 | 4.52 | 3.18 | -1.34 | 3.14 | -0.04 | -1.39 | -1.39 | 3.11 | -1.41 |
| Snap 3 | 4.19 | 3.67 | -0.52 | 3.62 | -0.05 | -0.57 | -0.57 | 3.57 | -0.62 |
| Snap 4 | 4.02 | 3.64 | -0.37 | 3.59 | -0.05 | -0.43 | -0.43 | 3.55 | -0.47 |
| Snap 5 | 4.26 | 4.01 | -0.24 | 3.97 | -0.04 | -0.29 | -0.29 | 3.95 | -0.31 |
| Snap 6 | 4.54 | 3.74 | -0.80 | 3.68 | -0.05 | -0.86 | -0.86 | 3.65 | -0.89 |
| Snap 7 | 4.53 | 4.27 | -0.26 | 4.23 | -0.04 | -0.30 | -0.30 | 4.18 | -0.35 |
| ∅ | 4.39 | 3.73 | -0.67 | 3.68 | -0.05 | -0.71 | -0.71 | 3.64 | -0.75 |

**Table S-2.4:** Excitation energies and contributions from the different polarization models to the $\mathcal{S}$-shifts and their average for different configurations of pNA in aug-cc-pVTZ quality and a 3 Å water environment obtained with a `PE` embedding model.

| $\Delta E^{\text{ex}}$(PE): | VACUUM | NOPOL | Δ NOPOL | GSPOL | ΔΔ GSPOL | DPOL | ΔΔ DPOL | ΔGSPOL | ΔDPOL | REF | Δ REF |
|---|---|---|---|---|---|---|---|---|---|---|---|
| Snap 1 | 4.68 | 3.56 | -1.12 | 3.52 | -0.05 | 3.49 | -0.02 | -1.17 | -1.19 | 3.50 | -1.19 |
| Snap 2 | 4.52 | 3.15 | -1.37 | 3.10 | -0.04 | 3.08 | -0.02 | -1.42 | -1.44 | 3.11 | -1.41 |
| Snap 3 | 4.19 | 3.65 | -0.54 | 3.60 | -0.06 | 3.56 | -0.04 | -0.60 | -0.63 | 3.57 | -0.62 |
| Snap 4 | 4.02 | 3.61 | -0.41 | 3.56 | -0.05 | 3.52 | -0.04 | -0.46 | -0.50 | 3.55 | -0.47 |
| Snap 5 | 4.26 | 4.00 | -0.25 | 3.96 | -0.04 | 3.94 | -0.03 | -0.29 | -0.32 | 3.95 | -0.31 |
| Snap 6 | 4.54 | 3.72 | -0.82 | 3.66 | -0.07 | 3.63 | -0.03 | -0.88 | -0.91 | 3.65 | -0.89 |
| Snap 7 | 4.53 | 4.26 | -0.27 | 4.22 | -0.04 | 4.20 | -0.03 | -0.31 | -0.33 | 4.18 | -0.35 |
| ∅ | 4.39 | 3.71 | -0.68 | 3.66 | -0.05 | 3.63 | -0.03 | -0.73 | -0.76 | 3.64 | -0.75 |

## S-2.2 Calculations in a 4 Å water environment

**Table S-2.5:** Excitation energies and contributions from the different polarization models to the $\mathcal{S}$-shifts and their average for different configurations of pNA in aug-cc-pVDZ quality and a 4 Å water environment obtained with a `FDE` embedding model.

| $\Delta E^{\text{ex}}$(FDE): | VACUUM | NOPOL | Δ NOPOL | GSPOL | ΔΔ GSPOL | ΔGSPOL | ΔDPOL | REF | Δ REF |
|---|---|---|---|---|---|---|---|---|---|
| Snap 1 | 4.68 | 3.49 | -1.18 | 3.43 | -0.07 | -1.25 | -1.25 | 3.38 | -1.30 |
| Snap 2 | 4.51 | 3.22 | -1.29 | 3.18 | -0.04 | -1.33 | -1.33 | 3.15 | -1.36 |
| Snap 3 | 4.19 | 3.57 | -0.61 | 3.50 | -0.07 | -0.68 | -0.68 | 3.43 | -0.76 |
| Snap 4 | 4.01 | 3.58 | -0.43 | 3.51 | -0.08 | -0.50 | -0.50 | 3.45 | -0.56 |
| Snap 5 | 4.25 | 4.01 | -0.24 | 3.96 | -0.05 | -0.29 | -0.29 | 3.93 | -0.32 |
| Snap 6 | 4.54 | 3.68 | -0.86 | 3.61 | -0.07 | -0.92 | -0.92 | 3.56 | -0.98 |
| Snap 7 | 4.53 | 4.22 | -0.31 | 4.17 | -0.05 | -0.36 | -0.36 | 4.10 | -0.43 |
| ∅ | 4.39 | 3.68 | -0.70 | 3.62 | -0.06 | -0.76 | -0.76 | 3.57 | -0.81 |

**Table S-2.6:** Excitation energies and contributions from the different polarization models to the $\mathcal{S}$-shifts and their average for different configurations of pNA in aug-cc-pVDZ quality and a 4 Å water environment obtained with a `PE` embedding model.

| $\Delta E^{\text{ex}}$(PE): | VACUUM | NOPOL | Δ NOPOL | GSPOL | ΔΔ GSPOL | DPOL | ΔΔ DPOL | ΔGSPOL | ΔDPOL | REF | Δ REF |
|---|---|---|---|---|---|---|---|---|---|---|---|
| Snap 1 | 4.68 | 3.49 | -1.19 | 3.41 | -0.08 | 3.38 | -0.03 | -1.26 | -1.30 | 3.38 | -1.30 |
| Snap 2 | 4.51 | 3.20 | -1.31 | 3.16 | -0.04 | 3.14 | -0.02 | -1.35 | -1.38 | 3.15 | -1.36 |
| Snap 3 | 4.19 | 3.57 | -0.62 | 3.47 | -0.09 | 3.41 | -0.06 | -0.71 | -0.77 | 3.43 | -0.76 |
| Snap 4 | 4.01 | 3.55 | -0.46 | 3.47 | -0.08 | 3.42 | -0.05 | -0.54 | -0.59 | 3.45 | -0.56 |
| Snap 5 | 4.25 | 4.00 | -0.25 | 3.96 | -0.04 | 3.92 | -0.04 | -0.30 | -0.33 | 3.93 | -0.32 |
| Snap 6 | 4.54 | 3.67 | -0.87 | 3.58 | -0.09 | 3.54 | -0.04 | -0.96 | -1.00 | 3.56 | -0.98 |
| Snap 7 | 4.53 | 4.22 | -0.31 | 4.16 | -0.06 | 4.12 | -0.04 | -0.37 | -0.41 | 4.10 | -0.43 |
| ∅ | 4.39 | 3.67 | -0.71 | 3.60 | -0.07 | 3.56 | -0.04 | -0.78 | -0.82 | 3.57 | -0.81 |

**Table S-2.7:** Excitation energies and contributions from the different polarization models to the $\mathcal{S}$-shifts and their average for different configurations of pNA in aug-cc-pVTZ quality and a 4 Å water environment obtained with a `FDE` embedding model.

| $\Delta E^{ex}$(FDE): | VACUUM | NOPOL | Δ NOPOL | GSPOL | ΔΔ GSPOL | ΔGSPOL | ΔDPOL | REF | Δ REF |
|---|---|---|---|---|---|---|---|---|---|
| Snap 1 | 4.68 | 3.51 | -1.18 | 3.44 | -0.07 | -1.25 | -1.25 | 3.40 | -1.29 |
| Snap 2 | 4.52 | 3.23 | -1.29 | 3.19 | -0.05 | -1.34 | -1.34 | 3.16 | -1.36 |
| Snap 3 | 4.19 | 3.58 | -0.62 | 3.50 | -0.07 | -0.69 | -0.69 | 3.44 | -0.75 |
| Snap 4 | 4.02 | 3.59 | -0.43 | 3.51 | -0.08 | -0.51 | -0.51 | 3.46 | -0.56 |
| Snap 5 | 4.26 | 4.02 | -0.24 | 3.97 | -0.05 | -0.29 | -0.29 | 3.94 | -0.32 |
| Snap 6 | 4.54 | 3.69 | -0.85 | 3.61 | -0.07 | -0.93 | -0.93 | 3.57 | -0.97 |
| Snap 7 | 4.53 | 4.23 | -0.31 | 4.17 | -0.05 | -0.36 | -0.36 | 4.11 | -0.42 |
| ∅ | 4.39 | 3.69 | -0.70 | 3.63 | -0.06 | -0.77 | -0.77 | 3.58 | -0.81 |

**Table S-2.8:** Excitation energies and contributions from the different polarization models to the $\mathcal{S}$-shifts and their average for different configurations of pNA in aug-cc-pVTZ quality and a 4 Å water environment obtained with a `PE` embedding model.

| $\Delta E^{ex}$(PE): | VACUUM | NOPOL | Δ NOPOL | GSPOL | ΔΔ GSPOL | DPOL | ΔΔ DPOL | ΔGSPOL | ΔDPOL | REF | Δ REF |
|---|---|---|---|---|---|---|---|---|---|---|---|
| Snap 1 | 4.68 | 3.50 | -1.18 | 3.42 | -0.08 | 3.39 | -0.03 | -1.26 | -1.30 | 3.40 | -1.29 |
| Snap 2 | 4.52 | 3.21 | -1.32 | 3.16 | -0.05 | 3.13 | -0.03 | -1.36 | -1.39 | 3.16 | -1.36 |
| Snap 3 | 4.19 | 3.57 | -0.62 | 3.47 | -0.10 | 3.41 | -0.06 | -0.72 | -0.78 | 3.44 | -0.75 |
| Snap 4 | 4.02 | 3.55 | -0.46 | 3.47 | -0.09 | 3.42 | -0.05 | -0.55 | -0.60 | 3.46 | -0.56 |
| Snap 5 | 4.26 | 4.01 | -0.24 | 3.96 | -0.05 | 3.93 | -0.04 | -0.29 | -0.33 | 3.94 | -0.32 |
| Snap 6 | 4.54 | 3.67 | -0.87 | 3.58 | -0.09 | 3.54 | -0.04 | -0.96 | -1.00 | 3.57 | -0.97 |
| Snap 7 | 4.53 | 4.23 | -0.31 | 4.17 | -0.06 | 4.13 | -0.04 | -0.37 | -0.41 | 4.11 | -0.42 |
| ∅ | 4.39 | 3.68 | -0.71 | 3.60 | -0.07 | 3.56 | -0.04 | -0.79 | -0.83 | 3.58 | -0.81 |

## S-2.3 PE calculations in a 5 Å water environment

**Table S-2.9:** Excitation energies and contributions from the different polarization models to the $\mathcal{S}$-shifts and their average for different configurations of pNA in aug-cc-pVDZ quality and a 5 Å water environment obtained with a `PE` embedding model.

| $\Delta E^{ex}$(PE): | VACUUM | NOPOL | Δ NOPOL | GSPOL | ΔΔ GSPOL | DPOL | ΔΔ DPOL | ΔGSPOL | ΔDPOL |
|---|---|---|---|---|---|---|---|---|---|
| Snap 1 | 4.68 | 3.44 | -1.23 | 3.35 | -0.09 | 3.31 | -0.04 | -1.33 | -1.36 |
| Snap 2 | 4.51 | 3.12 | -1.39 | 3.05 | -0.07 | 3.02 | -0.03 | -1.46 | -1.49 |
| Snap 3 | 4.19 | 3.53 | -0.66 | 3.41 | -0.11 | 3.35 | -0.06 | -0.77 | -0.84 |
| Snap 4 | 4.01 | 3.50 | -0.51 | 3.40 | -0.10 | 3.35 | -0.05 | -0.61 | -0.66 |
| Snap 5 | 4.25 | 3.99 | -0.27 | 3.93 | -0.05 | 3.90 | -0.03 | -0.32 | -0.36 |
| Snap 6 | 4.54 | 3.57 | -0.97 | 3.46 | -0.11 | 3.41 | -0.05 | -1.07 | -1.13 |
| Snap 7 | 4.53 | 4.22 | -0.30 | 4.16 | -0.06 | 4.12 | -0.04 | -0.36 | -0.40 |
| ∅ | 4.39 | 3.62 | -0.76 | 3.54 | -0.09 | 3.49 | -0.04 | -0.85 | -0.89 |

**Table S-2.10:** Excitation energies and contributions from the different polarization models to the $\mathcal{S}$-shifts and their average for different configurations of pNA in aug-cc-pVTZ quality and a 5 Å water environment obtained with a `PE` embedding model.

| $\Delta E^{\text{ex}}$(`PE`): | `VACUUM` | `NOPOL` | Δ `NOPOL` | `GSPOL` | ΔΔ `GSPOL` | `DPOL` | ΔΔ `DPOL` | Δ`GSPOL` | Δ`DPOL` |
|---|---|---|---|---|---|---|---|---|---|
| Snap 1 | 4.68 | 3.44 | -1.24 | 3.35 | -0.09 | 3.31 | -0.04 | -1.34 | -1.37 |
| Snap 2 | 4.52 | 3.12 | -1.40 | 3.05 | -0.07 | 3.02 | -0.03 | -1.47 | -1.50 |
| Snap 3 | 4.19 | 3.53 | -0.67 | 3.41 | -0.11 | 3.35 | -0.06 | -0.78 | -0.84 |
| Snap 4 | 4.02 | 3.50 | -0.51 | 3.40 | -0.10 | 3.35 | -0.05 | -0.61 | -0.67 |
| Snap 5 | 4.26 | 3.99 | -0.27 | 3.93 | -0.05 | 3.90 | -0.03 | -0.32 | -0.36 |
| Snap 6 | 4.54 | 3.57 | -0.97 | 3.46 | -0.11 | 3.41 | -0.05 | -1.08 | -1.13 |
| Snap 7 | 4.53 | 4.22 | -0.31 | 4.16 | -0.06 | 4.12 | -0.04 | -0.37 | -0.41 |
| ∅ | 4.39 | 3.62 | -0.77 | 3.54 | -0.09 | 3.49 | -0.04 | -0.85 | -0.90 |

## S-2.4 PE calculations in a 12 Å water environment

**Table S-2.11:** Excitation energies and contributions from the different polarization models to the $\mathcal{S}$-shifts and their average for different configurations of pNA in aug-cc-pVDZ quality and a 12 Å water environment obtained with a `PE` embedding model.

| $\Delta E^{\text{ex}}$(`PE`): | `VACUUM` | `NOPOL` | Δ `NOPOL` | `GSPOL` | ΔΔ `GSPOL` | `DPOL` | ΔΔ `DPOL` | Δ`GSPOL` | Δ`DPOL` |
|---|---|---|---|---|---|---|---|---|---|
| Snap 1 | 4.68 | 3.47 | -1.21 | 3.37 | -0.10 | 3.33 | -0.04 | -1.31 | -1.35 |
| Snap 2 | 4.51 | 3.08 | -1.44 | 2.94 | -0.13 | 2.90 | -0.04 | -1.57 | -1.61 |
| Snap 3 | 4.19 | 3.51 | -0.67 | 3.39 | -0.12 | 3.31 | -0.08 | -0.79 | -0.87 |
| Snap 4 | 4.01 | 3.33 | -0.69 | 3.17 | -0.15 | 3.10 | -0.07 | -0.84 | -0.91 |
| Snap 5 | 4.25 | 3.91 | -0.34 | 3.70 | -0.22 | 3.65 | -0.05 | -0.55 | -0.60 |
| Snap 6 | 4.54 | 3.54 | -1.00 | 3.40 | -0.13 | 3.34 | -0.06 | -1.13 | -1.19 |
| Snap 7 | 4.53 | 4.01 | -0.52 | 3.91 | -0.10 | 3.86 | -0.06 | -0.61 | -0.67 |
| ∅ | 4.39 | 3.55 | -0.84 | 3.41 | -0.14 | 3.36 | -0.06 | -0.97 | -1.03 |

**Table S-2.12:** Excitation energies and contributions from the different polarization models to the $\mathcal{S}$-shifts and their average for different configurations of pNA in aug-cc-pVTZ quality and a 12 Å water environment obtained with a `PE` embedding model.

| $\Delta E^{\text{ex}}$(`PE`): | `VACUUM` | `NOPOL` | Δ `NOPOL` | `GSPOL` | ΔΔ `GSPOL` | `DPOL` | ΔΔ `DPOL` | Δ`GSPOL` | Δ`DPOL` |
|---|---|---|---|---|---|---|---|---|---|
| Snap 1 | 4.68 | 3.49 | -1.20 | 3.38 | -0.11 | 3.33 | -0.04 | -1.31 | -1.35 |
| Snap 2 | 4.52 | 3.08 | -1.44 | 2.94 | -0.14 | 2.89 | -0.04 | -1.58 | -1.63 |
| Snap 3 | 4.19 | 3.52 | -0.67 | 3.39 | -0.13 | 3.31 | -0.08 | -0.80 | -0.88 |
| Snap 4 | 4.02 | 3.33 | -0.69 | 3.16 | -0.16 | 3.09 | -0.08 | -0.85 | -0.93 |
| Snap 5 | 4.26 | 3.93 | -0.33 | 3.71 | -0.22 | 3.66 | -0.05 | -0.55 | -0.60 |
| Snap 6 | 4.54 | 3.54 | -1.00 | 3.40 | -0.14 | 3.34 | -0.06 | -1.14 | -1.20 |
| Snap 7 | 4.53 | 4.02 | -0.51 | 3.92 | -0.10 | 3.86 | -0.06 | -0.61 | -0.67 |
| ∅ | 4.39 | 3.56 | -0.84 | 3.41 | -0.14 | 3.35 | -0.06 | -0.98 | -1.04 |

## S-2.5 Oscillator strengths and $\mathcal{F}$-shifts for *para*-nitroaniline

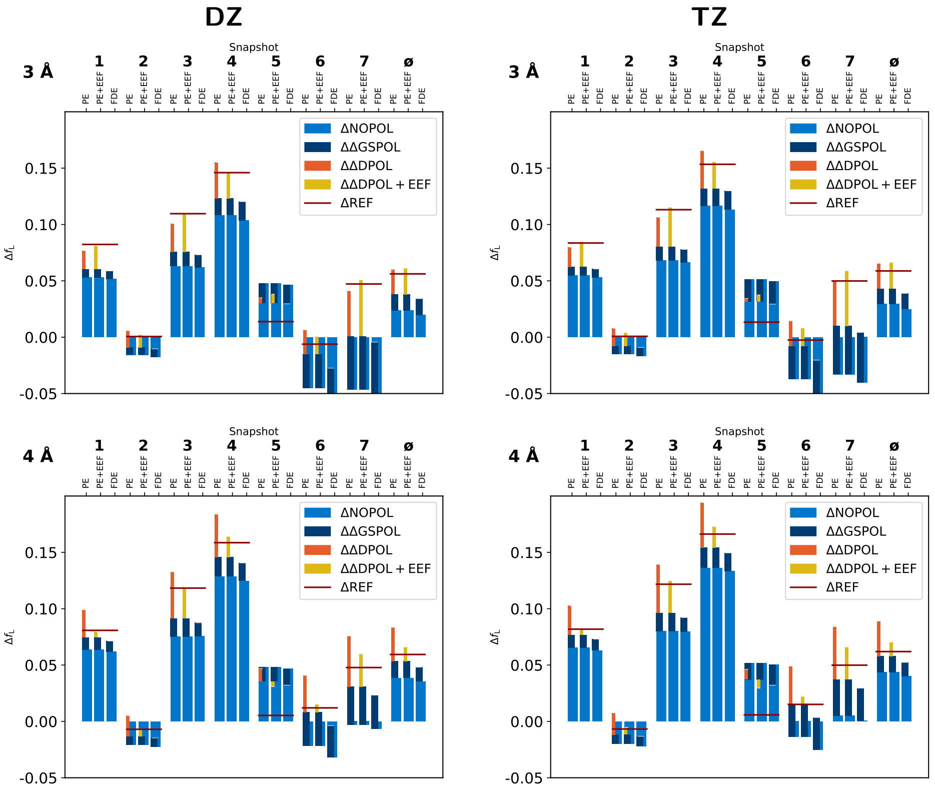


**Figure S-2.3:** Contributions to the $\mathcal{F}$-shifts and their average for different configurations of pNA in 3 and 4 Å water environments of water obtained from a MD simulation and subsequently calculated in a PE and FDE framework, different orders of polarization contributions and effective external field (EEF) effects obtained in calculations with aug-cc-pVDZ and aug-cc-pVTZ basis sets.

## S-2.6 Calculations in a 3 Å water environment

**Table S-2.13:** Oscillator strengths and contributions from the different polarization models to the $\mathcal{F}$-shifts and their average for different configurations of pNA in aug-cc-pVDZ quality and a 3 Å water environment obtained with a FDE embedding model.

| $\Delta f_L$ (FDE): | VACUUM | NOPOL | Δ NOPOL | GSPOL | ΔΔ GSPOL | ΔGSPOL | Δ DPOL | REF | Δ REF |
|---|---|---|---|---|---|---|---|---|---|
| Snap 1 | 0.129 | 0.180 | 0.052 | 0.187 | 0.007 | 0.059 | 0.059 | 0.211 | 0.082 |
| Snap 2 | 0.159 | 0.142 | -0.017 | 0.149 | 0.007 | -0.010 | -0.010 | 0.160 | 0.001 |
| Snap 3 | 0.301 | 0.362 | 0.062 | 0.374 | 0.011 | 0.073 | 0.073 | 0.410 | 0.110 |
| Snap 4 | 0.127 | 0.230 | 0.104 | 0.247 | 0.017 | 0.120 | 0.120 | 0.273 | 0.146 |
| Snap 5 | 0.261 | 0.307 | 0.046 | 0.291 | -0.017 | 0.030 | 0.030 | 0.275 | 0.014 |
| Snap 6 | 0.273 | 0.215 | -0.058 | 0.245 | 0.030 | -0.027 | -0.027 | 0.267 | -0.006 |
| Snap 7 | 0.306 | 0.255 | -0.051 | 0.301 | 0.046 | -0.004 | -0.004 | 0.353 | 0.047 |
| ∅ | 0.222 | 0.242 | 0.020 | 0.256 | 0.015 | 0.034 | 0.034 | 0.278 | 0.056 |

**Table S-2.14:** Oscillator strengths and contributions from the different polarization models to the $\mathcal{F}$-shifts and their average for different configurations of pNA in aug-cc-pVDZ quality and a 3 Å water environment obtained with a PE embedding model.

| $\Delta f_L$ (PE): | VACUUM | NOPOL | Δ NOPOL | GSPOL | ΔΔ GSPOL | DPOL | ΔΔ DPOL | DPOL+EEF | ΔΔ EEF | ΔGSPOL | ΔDPOL | ΔDPOL+EEF | REF | Δ REF |
|---|---|---|---|---|---|---|---|---|---|---|---|---|---|---|
| Snap 1 | 0.129 | 0.182 | 0.053 | 0.189 | 0.007 | 0.205 | 0.016 | 0.210 | 0.005 | 0.060 | 0.077 | 0.081 | 0.211 | 0.082 |
| Snap 2 | 0.159 | 0.143 | -0.016 | 0.150 | 0.007 | 0.165 | 0.015 | 0.162 | -0.004 | -0.009 | 0.006 | 0.003 | 0.160 | 0.001 |
| Snap 3 | 0.301 | 0.363 | 0.063 | 0.376 | 0.013 | 0.401 | 0.025 | 0.410 | 0.009 | 0.076 | 0.101 | 0.109 | 0.410 | 0.110 |
| Snap 4 | 0.127 | 0.235 | 0.108 | 0.250 | 0.015 | 0.282 | 0.032 | 0.273 | -0.009 | 0.123 | 0.155 | 0.146 | 0.273 | 0.146 |
| Snap 5 | 0.261 | 0.309 | 0.048 | 0.291 | -0.017 | 0.296 | 0.005 | 0.299 | 0.003 | 0.030 | 0.035 | 0.038 | 0.275 | 0.014 |
| Snap 6 | 0.273 | 0.228 | -0.045 | 0.258 | 0.030 | 0.279 | 0.022 | 0.273 | -0.006 | -0.015 | 0.007 | 0.000 | 0.267 | -0.006 |
| Snap 7 | 0.306 | 0.259 | -0.046 | 0.307 | 0.047 | 0.347 | 0.040 | 0.357 | 0.010 | 0.001 | 0.041 | 0.051 | 0.353 | 0.047 |
| ∅ | 0.222 | 0.246 | 0.024 | 0.260 | 0.014 | 0.282 | 0.022 | 0.283 | 0.001 | 0.038 | 0.060 | 0.061 | 0.278 | 0.056 |

**Table S-2.15:** Oscillator strengths and contributions from the different polarization models to the $\mathcal{F}$-shifts and their average for different configurations of pNA in aug-cc-pVTZ quality and a 3 Å water environment obtained with a FDE embedding model.

| $\Delta f_L$ (FDE): | VACUUM | NOPOL | Δ NOPOL | GSPOL | ΔΔ GSPOL | ΔGSPOL | ΔDPOL | REF | Δ REF |
|---|---|---|---|---|---|---|---|---|---|
| Snap 1 | 0.129 | 0.182 | 0.053 | 0.189 | 0.008 | 0.061 | 0.061 | 0.213 | 0.084 |
| Snap 2 | 0.160 | 0.143 | -0.017 | 0.151 | 0.008 | -0.009 | -0.009 | 0.161 | 0.001 |
| Snap 3 | 0.297 | 0.363 | 0.066 | 0.375 | 0.012 | 0.078 | 0.078 | 0.410 | 0.113 |
| Snap 4 | 0.119 | 0.233 | 0.113 | 0.249 | 0.017 | 0.130 | 0.130 | 0.273 | 0.153 |
| Snap 5 | 0.256 | 0.305 | 0.050 | 0.285 | -0.020 | 0.029 | 0.029 | 0.269 | 0.013 |
| Snap 6 | 0.271 | 0.219 | -0.051 | 0.250 | 0.031 | -0.020 | -0.020 | 0.268 | -0.003 |
| Snap 7 | 0.304 | 0.263 | -0.040 | 0.308 | 0.045 | 0.004 | 0.004 | 0.353 | 0.050 |
| ∅ | 0.219 | 0.244 | 0.025 | 0.258 | 0.014 | 0.039 | 0.039 | 0.278 | 0.059 |

**Table S-2.16:** Oscillator strengths and contributions from the different polarization models to the $\mathcal{F}$-shifts and their average for different configurations of pNA in aug-cc-pVTZ quality and a 3 Å water environment obtained with a PE embedding model.

| $\Delta f_L$ (PE): | VACUUM | NOPOL | Δ NOPOL | GSPOL | ΔΔ GSPOL | DPOL | ΔΔ DPOL | DPOL+EEF | ΔΔ EEF | ΔGSPOL | Δ DPOL | ΔDPOL+EEF | REF | Δ REF |
|---|---|---|---|---|---|---|---|---|---|---|---|---|---|---|
| Snap 1 | 0.129 | 0.184 | 0.055 | 0.191 | 0.008 | 0.209 | 0.017 | 0.213 | 0.004 | 0.063 | 0.080 | 0.084 | 0.213 | 0.084 |
| Snap 2 | 0.160 | 0.145 | -0.015 | 0.152 | 0.007 | 0.168 | 0.016 | 0.164 | -0.004 | -0.008 | 0.008 | 0.004 | 0.161 | 0.001 |
| Snap 3 | 0.297 | 0.365 | 0.068 | 0.377 | 0.012 | 0.404 | 0.026 | 0.412 | 0.008 | 0.080 | 0.106 | 0.115 | 0.410 | 0.113 |
| Snap 4 | 0.119 | 0.236 | 0.116 | 0.251 | 0.015 | 0.285 | 0.034 | 0.275 | -0.010 | 0.132 | 0.166 | 0.156 | 0.273 | 0.153 |
| Snap 5 | 0.256 | 0.307 | 0.051 | 0.287 | -0.020 | 0.290 | 0.003 | 0.293 | 0.003 | 0.031 | 0.034 | 0.037 | 0.269 | 0.013 |
| Snap 6 | 0.271 | 0.234 | -0.037 | 0.263 | 0.029 | 0.285 | 0.022 | 0.279 | -0.006 | -0.008 | 0.015 | 0.008 | 0.268 | -0.003 |
| Snap 7 | 0.304 | 0.271 | -0.033 | 0.314 | 0.043 | 0.354 | 0.040 | 0.363 | 0.009 | 0.010 | 0.050 | 0.059 | 0.353 | 0.050 |
| ∅ | 0.219 | 0.249 | 0.029 | 0.262 | 0.014 | 0.285 | 0.023 | 0.286 | 0.001 | 0.043 | 0.066 | 0.066 | 0.278 | 0.059 |

## S-2.7 Calculations in a 4 Å water environment

**Table S-2.17:** Oscillator strengths and contributions from the different polarization models to the $\mathcal{F}$-shifts and their average for different configurations of pNA in aug-cc-pVDZ quality and a 4 Å water environment obtained with a `FDE` embedding model.

| $\Delta f_L$ (FDE): | VACUUM | NOPOL | Δ NOPOL | GSPOL | ΔΔ GSPOL | Δ GSPOL | Δ DPOL | REF | Δ REF |
|---|---|---|---|---|---|---|---|---|---|
| Snap 1 | 0.129 | 0.190 | 0.062 | 0.200 | 0.010 | 0.071 | 0.071 | 0.209 | 0.081 |
| Snap 2 | 0.159 | 0.137 | -0.023 | 0.145 | 0.008 | -0.015 | -0.015 | 0.152 | -0.007 |
| Snap 3 | 0.301 | 0.376 | 0.076 | 0.388 | 0.012 | 0.088 | 0.088 | 0.419 | 0.118 |
| Snap 4 | 0.127 | 0.252 | 0.125 | 0.268 | 0.016 | 0.141 | 0.141 | 0.286 | 0.159 |
| Snap 5 | 0.261 | 0.308 | 0.047 | 0.293 | -0.014 | 0.032 | 0.032 | 0.266 | 0.005 |
| Snap 6 | 0.273 | 0.241 | -0.032 | 0.269 | 0.028 | -0.004 | -0.004 | 0.285 | 0.012 |
| Snap 7 | 0.306 | 0.299 | -0.006 | 0.329 | 0.030 | 0.023 | 0.023 | 0.354 | 0.048 |
| ∅ | 0.222 | 0.258 | 0.035 | 0.270 | 0.013 | 0.048 | 0.048 | 0.282 | 0.059 |

**Table S-2.18:** Oscillator strengths and contributions from the different polarization models to the $\mathcal{F}$-shifts and their average for different configurations of pNA in aug-cc-pVDZ quality and a 4 Å water environment obtained with a `PE` embedding model.

| $\Delta f_L$ (PE): | VACUUM | NOPOL | Δ NOPOL | GSPOL | ΔΔ GSPOL | DPOL | ΔΔ DPOL | DPOL+EEF | ΔΔ EEF | Δ GSPOL | ΔDPOL | Δ DPOL+EEF | REF | Δ REF |
|---|---|---|---|---|---|---|---|---|---|---|---|---|---|---|
| Snap 1 | 0.129 | 0.192 | 0.064 | 0.203 | 0.011 | 0.228 | 0.024 | 0.208 | -0.020 | 0.075 | 0.099 | 0.079 | 0.209 | 0.081 |
| Snap 2 | 0.159 | 0.139 | -0.021 | 0.146 | 0.007 | 0.164 | 0.018 | 0.152 | -0.012 | -0.013 | 0.005 | -0.007 | 0.152 | -0.007 |
| Snap 3 | 0.301 | 0.376 | 0.075 | 0.392 | 0.016 | 0.433 | 0.041 | 0.420 | -0.013 | 0.092 | 0.133 | 0.119 | 0.419 | 0.118 |
| Snap 4 | 0.127 | 0.256 | 0.129 | 0.273 | 0.017 | 0.311 | 0.038 | 0.291 | -0.020 | 0.146 | 0.184 | 0.164 | 0.286 | 0.159 |
| Snap 5 | 0.261 | 0.309 | 0.048 | 0.297 | -0.013 | 0.308 | 0.011 | 0.292 | -0.016 | 0.036 | 0.047 | 0.031 | 0.266 | 0.005 |
| Snap 6 | 0.273 | 0.251 | -0.022 | 0.281 | 0.030 | 0.314 | 0.033 | 0.288 | -0.026 | 0.008 | 0.041 | 0.015 | 0.285 | 0.012 |
| Snap 7 | 0.306 | 0.303 | -0.003 | 0.336 | 0.034 | 0.382 | 0.045 | 0.366 | -0.016 | 0.031 | 0.076 | 0.060 | 0.354 | 0.048 |
| ∅ | 0.222 | 0.261 | 0.039 | 0.275 | 0.015 | 0.306 | 0.030 | 0.288 | -0.018 | 0.053 | 0.083 | 0.066 | 0.282 | 0.059 |

**Table S-2.19:** Oscillator strengths and contributions from the different polarization models to the $\mathcal{F}$-shifts and their average for different configurations of pNA in aug-cc-pVTZ quality and a 4 Å water environment obtained with a `FDE` embedding model.

| $\Delta f_L$ (FDE): | VACUUM | NOPOL | Δ NOPOL | GSPOL | ΔΔ GSPOL | ΔGSPOL | ΔDPOL | REF | Δ REF |
|---|---|---|---|---|---|---|---|---|---|
| Snap 1 | 0.129 | 0.192 | 0.063 | 0.202 | 0.010 | 0.073 | 0.073 | 0.211 | 0.082 |
| Snap 2 | 0.160 | 0.138 | -0.022 | 0.147 | 0.009 | -0.013 | -0.013 | 0.153 | -0.007 |
| Snap 3 | 0.297 | 0.377 | 0.080 | 0.389 | 0.013 | 0.092 | 0.092 | 0.419 | 0.122 |
| Snap 4 | 0.119 | 0.253 | 0.133 | 0.269 | 0.016 | 0.150 | 0.150 | 0.286 | 0.166 |
| Snap 5 | 0.256 | 0.306 | 0.050 | 0.288 | -0.018 | 0.032 | 0.032 | 0.261 | 0.006 |
| Snap 6 | 0.271 | 0.246 | -0.025 | 0.274 | 0.028 | 0.003 | 0.003 | 0.286 | 0.015 |
| Snap 7 | 0.304 | 0.304 | 0.001 | 0.333 | 0.029 | 0.030 | 0.030 | 0.353 | 0.050 |
| ∅ | 0.219 | 0.259 | 0.040 | 0.272 | 0.012 | 0.052 | 0.052 | 0.281 | 0.062 |

**Table S-2.20:** Oscillator strengths and contributions from the different polarization models to the $\mathcal{F}$-shifts and their average for different configurations of pNA in aug-cc-pVTZ quality and a 4 Å water environment obtained with a `PE` embedding model.

| $\Delta f_L$ (PE): | VACUUM | NOPOL | Δ NOPOL | GSPOL | ΔΔ GSPOL | DPOL | ΔΔ DPOL | DPOL+EEF | ΔΔ EEF | ΔGSPOL | ΔDPOL | ΔDPOL+EEF | REF | Δ REF |
|---|---|---|---|---|---|---|---|---|---|---|---|---|---|---|
| Snap 1 | 0.129 | 0.194 | 0.065 | 0.206 | 0.011 | 0.232 | 0.026 | 0.211 | -0.021 | 0.077 | 0.103 | 0.082 | 0.211 | 0.082 |
| Snap 2 | 0.160 | 0.140 | -0.020 | 0.148 | 0.008 | 0.167 | 0.019 | 0.155 | -0.012 | -0.012 | 0.008 | -0.005 | 0.153 | -0.007 |
| Snap 3 | 0.297 | 0.377 | 0.080 | 0.394 | 0.016 | 0.436 | 0.043 | 0.422 | -0.014 | 0.096 | 0.139 | 0.125 | 0.419 | 0.122 |
| Snap 4 | 0.119 | 0.256 | 0.136 | 0.274 | 0.018 | 0.314 | 0.040 | 0.292 | -0.022 | 0.154 | 0.194 | 0.173 | 0.286 | 0.166 |
| Snap 5 | 0.256 | 0.307 | 0.052 | 0.293 | -0.015 | 0.302 | 0.009 | 0.285 | -0.017 | 0.037 | 0.046 | 0.029 | 0.261 | 0.006 |
| Snap 6 | 0.271 | 0.257 | -0.014 | 0.286 | 0.029 | 0.320 | 0.034 | 0.293 | -0.027 | 0.015 | 0.049 | 0.022 | 0.286 | 0.015 |
| Snap 7 | 0.304 | 0.309 | 0.005 | 0.341 | 0.032 | 0.388 | 0.047 | 0.370 | -0.018 | 0.037 | 0.084 | 0.066 | 0.353 | 0.050 |
| ∅ | 0.219 | 0.263 | 0.044 | 0.277 | 0.014 | 0.308 | 0.031 | 0.290 | -0.019 | 0.058 | 0.089 | 0.070 | 0.281 | 0.062 |

## S-2.8 PE calculations in aug-cc-pVDZ quality in a 5 Å water environment

**Table S-2.21:** Oscillator strengths and contributions from the different polarization models to the $\mathcal{F}$-shifts and their average for different configurations of pNA in aug-cc-pVDZ quality and a 5 Å water environment obtained with a PE embedding model.

| $\Delta f_L$ (PE): | VACUUM | NOPOL | Δ NOPOL | GSPOL | ΔΔ GSPOL | DPOL | ΔΔ DPOL | ΔGSPOL | ΔDPOL |
|---|---|---|---|---|---|---|---|---|---|
| Snap 1 | 0.129 | 0.199 | 0.070 | 0.211 | 0.012 | 0.239 | 0.028 | 0.082 | 0.110 |
| Snap 2 | 0.159 | 0.152 | -0.007 | 0.163 | 0.011 | 0.185 | 0.022 | 0.004 | 0.026 |
| Snap 3 | 0.301 | 0.381 | 0.081 | 0.401 | 0.019 | 0.446 | 0.045 | 0.100 | 0.146 |
| Snap 4 | 0.127 | 0.263 | 0.136 | 0.281 | 0.018 | 0.322 | 0.042 | 0.154 | 0.195 |
| Snap 5 | 0.261 | 0.303 | 0.041 | 0.268 | -0.035 | 0.257 | -0.011 | 0.007 | -0.004 |
| Snap 6 | 0.273 | 0.278 | 0.005 | 0.303 | 0.025 | 0.341 | 0.038 | 0.030 | 0.069 |
| Snap 7 | 0.306 | 0.297 | -0.009 | 0.335 | 0.038 | 0.383 | 0.049 | 0.029 | 0.078 |
| ∅ | 0.222 | 0.268 | 0.045 | 0.280 | 0.013 | 0.311 | 0.030 | 0.058 | 0.088 |

**Table S-2.22:** Oscillator strengths and contributions from the different polarization models to the $\mathcal{F}$-shifts and their average for different configurations of pNA in aug-cc-pVTZ quality and a 5 Å water environment obtained with a PE embedding model.

| $\Delta f_L$ (PE): | VACUUM | NOPOL | Δ NOPOL | GSPOL | ΔΔ GSPOL | DPOL | ΔΔ DPOL | ΔGSPOL | ΔDPOL |
|---|---|---|---|---|---|---|---|---|---|
| Snap 1 | 0.129 | 0.199 | 0.070 | 0.211 | 0.012 | 0.239 | 0.028 | 0.082 | 0.110 |
| Snap 2 | 0.160 | 0.152 | -0.008 | 0.163 | 0.011 | 0.185 | 0.022 | 0.003 | 0.025 |
| Snap 3 | 0.297 | 0.381 | 0.084 | 0.401 | 0.019 | 0.446 | 0.045 | 0.104 | 0.149 |
| Snap 4 | 0.119 | 0.263 | 0.144 | 0.281 | 0.018 | 0.322 | 0.042 | 0.161 | 0.203 |
| Snap 5 | 0.256 | 0.303 | 0.047 | 0.268 | -0.035 | 0.257 | -0.011 | 0.012 | 0.002 |
| Snap 6 | 0.271 | 0.278 | 0.008 | 0.303 | 0.025 | 0.341 | 0.038 | 0.033 | 0.071 |
| Snap 7 | 0.304 | 0.297 | -0.007 | 0.335 | 0.038 | 0.383 | 0.049 | 0.031 | 0.080 |
| ∅ | 0.219 | 0.268 | 0.048 | 0.280 | 0.013 | 0.311 | 0.030 | 0.061 | 0.091 |

## S-2.9 PE calculations in aug-cc-pVDZ quality in a 12 Å water environment

**Table S-2.23:** Oscillator strengths and contributions from the different polarization models to the $\mathcal{F}$-shifts and their average for different configurations of pNA in aug-cc-pVDZ quality and a 12 Å water environment obtained with a PE embedding model.

| $\Delta f_L$ (PE): | VACUUM | NOPOL | Δ NOPOL | GSPOL | ΔΔ GSPOL | DPOL | ΔΔ DPOL | ΔGSPOL | ΔDPOL |
|---|---|---|---|---|---|---|---|---|---|
| Snap 1 | 0.129 | 0.194 | 0.065 | 0.207 | 0.013 | 0.239 | 0.032 | 0.079 | 0.111 |
| Snap 2 | 0.159 | 0.158 | -0.001 | 0.177 | 0.019 | 0.205 | 0.027 | 0.018 | 0.045 |
| Snap 3 | 0.301 | 0.382 | 0.082 | 0.403 | 0.021 | 0.457 | 0.054 | 0.102 | 0.156 |
| Snap 4 | 0.127 | 0.289 | 0.162 | 0.311 | 0.022 | 0.362 | 0.050 | 0.184 | 0.235 |
| Snap 5 | 0.261 | 0.236 | -0.026 | 0.230 | -0.005 | 0.314 | 0.084 | -0.031 | 0.053 |
| Snap 6 | 0.273 | 0.286 | 0.013 | 0.313 | 0.027 | 0.358 | 0.045 | 0.040 | 0.085 |
| 078 Snap 7 | 0.306 | 0.355 | 0.049 | 0.365 | 0.011 | 0.419 | 0.053 | 0.060 | 0.113 |
| ∅ | 0.222 | 0.271 | 0.049 | 0.287 | 0.015 | 0.336 | 0.049 | 0.065 | 0.114 |

**Table S-2.24:** Oscillator strengths and contributions from the different polarization models to the $\mathcal{F}$-shifts and their average for different configurations of pNA in aug-cc-pVTZ quality and a 12 Å water environment obtained with a PE embedding model.

| $\Delta f_L$ (PE): | VACUUM | NOPOL | Δ NOPOL | GSPOL | ΔΔ GSPOL | DPOL | ΔΔ DPOL | ΔGSPOL | ΔDPOL |
|---|---|---|---|---|---|---|---|---|---|
| Snap 1 | 0.129 | 0.196 | 0.067 | 0.210 | 0.014 | 0.244 | 0.034 | 0.081 | 0.115 |
| Snap 2 | 0.160 | 0.160 | 0.000 | 0.179 | 0.020 | 0.208 | 0.029 | 0.020 | 0.048 |
| Snap 3 | 0.297 | 0.383 | 0.086 | 0.404 | 0.021 | 0.460 | 0.056 | 0.107 | 0.163 |
| Snap 4 | 0.119 | 0.289 | 0.170 | 0.313 | 0.023 | 0.366 | 0.053 | 0.193 | 0.246 |
| Snap 5 | 0.256 | 0.232 | -0.024 | 0.237 | 0.005 | 0.324 | 0.087 | -0.018 | 0.068 |
| Snap 6 | 0.271 | 0.289 | 0.018 | 0.315 | 0.026 | 0.362 | 0.047 | 0.045 | 0.091 |
| Snap 7 | 0.304 | 0.357 | 0.053 | 0.368 | 0.011 | 0.424 | 0.056 | 0.064 | 0.120 |
| ∅ | 0.219 | 0.272 | 0.053 | 0.289 | 0.017 | 0.341 | 0.052 | 0.070 | 0.122 |

# S-3 Shifts of pentameric formyl thiophene acetic acid

## S-3.1 Excitation energies and $\mathcal{S}$-shifts of pentameric formyl thiophene acetic acid in a 3 Å water environment in aug-cc-pVDZ quality

**Table S-3.1:** Excitation energies and contributions from the different polarization models to the $\mathcal{S}$-shifts and their average for different configurations of pFTAA in aug-cc-pVDZ quality and a 3 Å water environment obtained with a FDE embedding model.

| $\Delta E^{ex}$(FDE): | VACUUM | NOPOL | Δ NOPOL | GSPOL | ΔΔ GSPOL | ΔGSPOL | ΔDPOL | REF | ΔREF |
|---|---|---|---|---|---|---|---|---|---|
| Snap 1 | 2.92 | 3.07 | 0.15 | 3.09 | 0.01 | 0.17 | 0.17 | 3.05 | 0.14 |
| Snap 2 | 3.17 | 3.21 | 0.04 | 3.24 | 0.02 | 0.07 | 0.07 | 3.20 | 0.03 |
| ∅ | 3.05 | 3.14 | 0.10 | 3.16 | 0.02 | 0.12 | 0.12 | 3.13 | 0.09 |

**Table S-3.2:** Excitation energies and contributions from the different polarization models to the $\mathcal{S}$-shifts and their average for different configurations of pFTAA in aug-cc-pVDZ quality and a 3 Å water environment obtained with a PE embedding model and pseudo-potentials for entries marked with $^*$.

| $\Delta E^{ex}$(PE): | VACUUM | NOPOL | Δ NOPOL | GSPOL | ΔΔ GSPOL | DPOL | ΔΔ DPOL | ΔGSPOL | ΔDPOL | REF | ΔREF |
|---|---|---|---|---|---|---|---|---|---|---|---|
| Snap 1 | 2.92 | 3.08 | 0.16 | 3.09 | 0.01 | 3.06 | -0.03 | 0.17 | 0.14 | 3.05 | 0.14 |
| Snap 2$^*$ | 3.17 | 3.18 | 0.01 | 3.24 | 0.05 | 3.16 | -0.08 | 0.07 | -0.02 | 3.20 | 0.03 |
| Snap 3$^*$ | 2.78 | 2.68 | -0.09 | 2.85 | 0.17 | 2.82 | -0.03 | 0.07 | 0.04 | 2.64 | -0.13 |
| Snap 4$^*$ | 2.98 | 2.90 | -0.08 | 2.97 | 0.07 | 2.95 | -0.02 | -0.01 | -0.04 | 2.90 | -0.09 |
| Snap 5 | 3.20 | 3.31 | 0.11 | 3.32 | 0.02 | 3.29 | -0.04 | 0.13 | 0.09 | 3.28 | 0.08 |
| Snap 6 | 3.36 | 3.46 | 0.10 | 3.46 | 0.00 | 3.43 | -0.03 | 0.10 | 0.07 | 3.42 | 0.06 |
| Snap 7 | 2.74 | 2.80 | 0.06 | 2.83 | 0.03 | 2.79 | -0.04 | 0.09 | 0.05 | 2.80 | 0.06 |
| Snap 8$^*$ | 3.05 | 2.91 | -0.14 | 2.95 | 0.03 | 2.91 | -0.03 | -0.10 | -0.14 | 2.95 | -0.10 |
| ∅ | 3.02 | 3.04 | 0.02 | 3.09 | 0.05 | 3.05 | -0.04 | 0.07 | 0.03 | 3.03 | 0.01 |

## S-3.2 Oscillator strengths and $\mathcal{F}$-shifts of pFTAA in a 3 Å water environment in aug-cc-pVDZ quality

**Table S-3.3:** Oscillator strengths and contributions from the different polarization models to the $\mathcal{F}$-shifts and their average for different configurations of pFTAA in aug-cc-pVDZ quality in a 3 Å water environment obtained with a `FDE` embedding model.

| $f_L$ (FDE): | VACUUM | NOPOL | Δ NOPOL | GSPOL | ΔΔ GSPOL | ΔGSPOL | ΔDPOL | REF | ΔREF |
|---|---|---|---|---|---|---|---|---|---|
| Snap 1 | 0.900 | 1.195 | 0.294 | 1.248 | 0.053 | 0.348 | 0.348 | 1.288 | 0.388 |
| Snap 2 | 1.165 | 1.304 | 0.140 | 1.348 | 0.044 | 0.183 | 0.183 | 1.157 | -0.007 |
| ∅ | 1.033 | 1.249 | 0.217 | 1.298 | 0.049 | 0.265 | 0.265 | 1.223 | 0.191 |

**Table S-3.4:** Oscillator strengths and contributions from the different polarization models to the $\mathcal{F}$-shifts and their average for different configurations of pFTAA in aug-cc-pVDZ quality in a 3 Å water environment obtained with a `PE` embedding model (and optional effective external potential (EEF)) and pseudo-potentials for entries marked with $^*$.

| $\Delta f_L$ (PE): | VACUUM | NOPOL | Δ NOPOL | GSPOL | ΔΔ GSPOL | DPOL | ΔΔ DPOL | DPOL+EEF | ΔΔ EEF | ΔGSPOL | ΔDPOL | ΔDPOL+EEF | REF | ΔREF |
|---|---|---|---|---|---|---|---|---|---|---|---|---|---|---|
| Snap 1 | 0.900 | 1.221 | 0.320 | 1.280 | 0.060 | 1.343 | 0.063 | 1.314 | -0.029 | 0.380 | 0.443 | 0.414 | 1.288 | 0.388 |
| Snap 2* | 1.165 | 1.308 | 0.143 | 1.332 | 0.024 | 1.384 | 0.052 | 1.308 | -0.076 | 0.167 | 0.219 | 0.143 | 1.157 | -0.007 |
| Snap 3* | 1.150 | 1.076 | -0.074 | 1.226 | 0.150 | 1.284 | 0.058 | 1.212 | -0.072 | 0.076 | 0.134 | 0.0617 | 1.086 | -0.064 |
| Snap 4* | 1.214 | 1.089 | -0.125 | 1.197 | 0.108 | 1.274 | 0.078 | 1.214 | -0.060 | -0.017 | 0.061 | -0.0001 | 1.065 | -0.148 |
| Snap 5 | 1.242 | 1.439 | 0.197 | 1.472 | 0.034 | 1.556 | 0.084 | 1.518 | -0.038 | 0.231 | 0.315 | 0.276 | 1.504 | 0.263 |
| Snap 6 | 0.802 | 1.299 | 0.497 | 1.350 | 0.000 | 1.422 | 0.071 | 1.348 | -0.074 | 0.548 | 0.620 | 0.546 | 1.274 | 0.472 |
| Snap 7 | 1.094 | 1.282 | 0.188 | 1.358 | 0.077 | 1.420 | 0.061 | 1.352 | -0.068 | 0.265 | 0.326 | 0.258 | 1.340 | 0.246 |
| Snap 8* | 1.359 | 1.470 | 0.111 | 1.500 | 0.030 | 1.534 | 0.034 | 1.440 | -0.094 | 0.141 | 0.175 | 0.081 | 1.416 | 0.057 |
| ∅ | 1.116 | 1.273 | 0.157 | 1.339 | 0.060 | 1.402 | 0.063 | 1.338 | -0.064 | 0.224 | 0.287 | 0.222 | 1.266 | 0.151 |
